# Supplementary material for: Spatial Decompositions for Large Scale SVMs
Source: arXiv:1612.00374 source file (2018-02-08)
Supplement: Supplementary file 1 [file supplement.tex]

\documentclass{article}

% if you need to pass options to natbib, use, e.g.:
% \PassOptionsToPackage{numbers, compress}{natbib}
% before loading nips_2016
%
% to avoid loading the natbib package, add option nonatbib:
% \usepackage[nonatbib]{nips_2016}

\usepackage{nips_2016}

% to compile a camera-ready version, add the [final] option, e.g.:
% \usepackage[final]{nips_2016}

\usepackage[utf8]{inputenc} % allow utf-8 input
\usepackage[T1]{fontenc}    % use 8-bit T1 fonts
\usepackage{hyperref}       % hyperlinks
\usepackage{url}            % simple URL typesetting
\usepackage{booktabs}       % professional-quality tables
\usepackage{amsfonts}       % blackboard math symbols
\usepackage{nicefrac}       % compact symbols for 1/2, etc.
\usepackage{microtype}      % microtypography

\usepackage{xr}
\externaldocument{master}

\newlength{\myleftmargin}
\setlength{\myleftmargin}{-5ex}

\input{macros}
\input{local-macros}

\title{Spatial Decompositions for Large Scale SVMs, Supplementary Material}

% The \author macro works with any number of authors. There are two
% commands used to separate the names and addresses of multiple
% authors: \And and \AND.
%
% Using \And between authors leaves it to LaTeX to determine where to
% break the lines. Using \AND forces a line break at that point. So,
% if LaTeX puts 3 of 4 authors names on the first line, and the last
% on the second line, try using \AND instead of \And before the third
% author name.

\author{
  Philipp Thomann \\
  Institut für Stochastik und Anwendungen\\
  Universität Stuttgart \\
  Pfaffenwaldring 57, 70569 Stuttgart \\
  \texttt{philipp.thomann@mathematik.uni-stuttgart.de}\\
  \And
  Ingo Steinwart \\ %% \thanks{}
  Institut für Stochastik und Anwendungen\\
  Universität Stuttgart \\
  Pfaffenwaldring 57, 70569 Stuttgart \\
  \texttt{ingo.steinwart@mathematik.uni-stuttgart.de}
  %% examples of more authors
  \And
  Ingrid Blaschzyk \\
  Institut für Stochastik und Anwendungen\\
  Universität Stuttgart \\
  Pfaffenwaldring 57, 70569 Stuttgart \\
  \texttt{ingrid.blaschzyk@mathematik.uni-stuttgart.de}\\
  \And
  Mona Meister \\
  Robert Bosch GmbH \\
  70442 Stuttgart \\
  \texttt{mona.meister@de.bosch.com}\\
  %% Affiliation \\
  %% Address \\
  %% \texttt{email} \\
  %% \AND
  %% Coauthor \\
  %% Affiliation \\
  %% Address \\
  %% \texttt{email} \\
  %% \And
  %% Coauthor \\
  %% Affiliation \\
  %% Address \\
  %% \texttt{email} \\
  %% \And
  %% Coauthor \\
  %% Affiliation \\
  %% Address \\
  %% \texttt{email} \\
}

\begin{document}
% \nipsfinalcopy is no longer used

\maketitle

\appendix

\section{Proofs}
\input{theory_proof}

\section{Appendix}
\input{theory_appendix}

\input{more_results}

\section{More References on Large Scale SVMs}

For completeness we give here more References:
\begin{enumerate}
\item Sequential Minimal Optimization \cite{Platt99a,HsLi02a, GlIg06a, StHuSc11a},
\item parallel solvers \cite{CoBeBe02a,GrCoBoVa04a,DuCoGr07a, ZhWaBaLiQiCuCh08a, MeBiWe14a,TyGaWeAgTrXXa},
\item GPU-based solvers \cite{CaSuKe08a,Carpenter09a, CoSrKe11a,TyGaWeAgTrXXa},
%%%% TyGaWeAgTrXXa already cited before ||
\item FPGA-based approaches \cite{DuCoGrCaJaChMa12a,MaCaBeChGr12a},
\item matrix approximations \cite{WiSe01a,DrMa05a,KuMoTa12a,RudiCamorianoRosasco2015,SuZhZh15a},
\item kernel function approximations \cite{YaDuGuDa03a,RaDu07a,RaRe08a,FaChHsWaLi08a,SSSiSrCo11a,NiHuHu14a,HuAvSaSiRa14a, LuMaLiGaGuBeFaCoKiPiShXXa},
\item iterative strategies: \cite{RoVi15a,LiRoZh15a}.
\end{enumerate}

More references for decomposition strategies:
\begin{enumerate}
\item Random chunks: \cite{ChawlaEschrichHall2000,ChawlaHallBowyerKegelmeyer2004,ClaesenEtAl2014}:
\item robust learning from random bites \cite{ChristmannSteinwartHubert2007,Christmann2005b}.
\item clusters: \cite{ChTaJi07a,ChTaJi10a},
\item decision trees: \cite{BeBl98a, WuBeCrST99a, ChGuLiLu10a},
\item $k$-nearest neighbors: \cite{ZhBeMaMa06a, BlBr07b, BlBr07a, BlMe08a, SeBl08a, SeBl10a, Hable13a}.
\end{enumerate}

\small

\bibliographystyle{plain}

\small

\bibliography{bib/additional,bib/steinwart-books,bib/steinwart-proc,bib/steinwart-article,bib/steinwart-mine,bib/christmann}

\end{document}
